# Supplementary material for: Audio-Visual Class-Incremental Learning for Fish Feeding intensity Assessment in Aquaculture
Source: arXiv:2504.15171 source file (2025-04-21)
Supplement: Supplementary file 1 [file Appendix.tex]

\section{Hierarchical Representation Learning Structure}
The formula $W_{int} = (F_{av}^T F_{av} + \eta I)^{-1} F_{av}^T Y$ is derived from solving a regularized least squares optimization problem. Let me walk you through the complete derivation process:

We begin with a standard supervised learning objective: finding weights $W_{int}$ that minimize the squared error between predictions and true labels, with an additional regularization term to prevent overfitting:

\begin{equation}
\min_{W_{int}} \|Y - F_{av}W_{int}\|_F^2 + \eta\|W_{int}\|_F^2
\end{equation}

where:
- $F_{av}$ is the matrix of fused audio-visual features from training data (size $n \times d$, with $n$ samples and $d$ features)
- $Y$ is the matrix of intensity labels encoded as one-hot vectors (size $n \times c$, with $c$ intensity classes)
- $\|\cdot\|_F$ denotes the Frobenius norm
- $\eta$ is the regularization parameter

Let's expand the objective function:

\begin{equation}
\begin{aligned}
J(W_{int}) &= \|Y - F_{av}W_{int}\|_F^2 + \eta\|W_{int}\|_F^2 \\
&= \text{Tr}[(Y - F_{av}W_{int})^T(Y - F_{av}W_{int})] + \eta \text{Tr}[W_{int}^T W_{int}] \\
&= \text{Tr}[Y^TY - Y^TF_{av}W_{int} - W_{int}^TF_{av}^TY + W_{int}^TF_{av}^TF_{av}W_{int}] + \eta \text{Tr}[W_{int}^T W_{int}]
\end{aligned}
\end{equation}

where $\text{Tr}[\cdot]$ denotes the trace of a matrix.

To find the minimum, we take the derivative of the objective function with respect to $W_{int}$ and set it to zero:

\begin{equation}
\begin{aligned}
\frac{\partial J(W_{int})}{\partial W_{int}} &= \frac{\partial}{\partial W_{int}}[\text{Tr}[Y^TY - Y^TF_{av}W_{int} - W_{int}^TF_{av}^TY + W_{int}^TF_{av}^TF_{av}W_{int} + \eta W_{int}^T W_{int}]] \\
&= -F_{av}^TY - F_{av}^TY + 2F_{av}^TF_{av}W_{int} + 2\eta W_{int} \\
&= -2F_{av}^TY + 2(F_{av}^TF_{av} + \eta I)W_{int}
\end{aligned}
\end{equation}

Here, I've used matrix calculus identities such as:
- $\frac{\partial}{\partial X}\text{Tr}[AX] = A^T$
- $\frac{\partial}{\partial X}\text{Tr}[X^TAX] = 2AX$ (when $A$ is symmetric)

Setting the derivative to zero:

\begin{equation}
\begin{aligned}
-2F_{av}^TY + 2(F_{av}^TF_{av} + \eta I)W_{int} &= 0 \\
(F_{av}^TF_{av} + \eta I)W_{int} &= F_{av}^TY
\end{aligned}
\end{equation}

Finally, we solve for $W_{int}$:

\begin{equation}
W_{int} = (F_{av}^TF_{av} + \eta I)^{-1}F_{av}^TY
\end{equation}

This is the closed-form solution to the regularized least squares problem, often called ridge regression. The term $(F_{av}^TF_{av} + \eta I)^{-1}F_{av}^T$ is known as the pseudo-inverse of $F_{av}$ with regularization.

The correlation matrix $R = (F_{av}^TF_{av} + \eta I)^{-1}$ is preserved because it's needed for recursive updates in incremental learning without storing previous data. This is why we separate the formula into $W_{int} = R \cdot F_{av}^TY$ for computational efficiency in the incremental learning setting.
